# Supplementary material for: Matina: A Large-Scale 73B Token Persian Text Corpus
Source: arXiv:2502.09188 source file (2025-02-13)
Supplement: Supplementary file 1 [file appendixMain.tex]

\section{Detailed Preprocessing and Deduplication Pipelines}
\input{./appendix1_web}
\input{./appendix1_book}
